# Supplementary material for: Game-Theoretic Planning for Autonomous Driving among Risk-Aware Human Drivers
Source: arXiv:2205.00562 source file (2022-05-01)
Supplement: Supplementary file 1 [file appendixA.tex]

\section{More details of Approach}
\label{app: summary_of_approach}
% \subsection{Summary}
\input{NeuRIPS2020/Tables/centrality_cmetric}

\begin{enumerate}
    \item Obtain the positions of all vehicles using sensors deployed on the autonomous vehicle and form Dynamic Geometric Graphs (Section~\ref{subsec: DGG}).
    
    % \item At each time instance, we compute the Laplacian matrix $L_t$ using Equation~\ref{eq: Lt}.
    
    \item Compute the closeness and degree centrality function values using the definitions in Section~\ref{subsec: background_centrality}.
    
    \item Use the CMetric value to measure the likelihood and intensity of specific driving styles listed in Table~\ref{tab: behaviors_centrality}.
    
    % \item Perform clustering on the centrality function values to classify vehicles according to different behaviors. Each behavior corresponds to a different cluster (Section~\ref{subsec: clustering}).
    
\end{enumerate}

\begin{algorithm}
    \SetKwInOut{Input}{Input}
    \SetKwInOut{Output}{Output}
\SetKwComment{Comment}{$\triangleright$\ }{}
\SetAlgoLined
\Input{$u = v_i \gets [x_i,y_i]^\top \ \forall v_i \in \mathcal{V}(t)$}
\Output{$\textrm{SLE}(t), \textrm{SIE}(t)$}
$t=0$\\
\For {each $v \in \mathcal{V}(t)$}{
\While{$t \leq T$}{ 
// Compute Centrality //\\
$     \zeta^i_c[t] = \frac{N-1}{\sum_{v_j\in \mathcal{V}(t)\setminus \{v_i\}} \mc{D}_t(v_i,v_j)}$ \\ 
$    \zeta^i_d[t] = \bigl | \{ v_j \in \mc{N}_i(t) \} \bigr | \ \textrm{such that} (v_i,v_j) \not\in \mc{E(\tau)}, \tau = 0, \ldots, t-1$ \\
$         \zeta^i_e[t] = \frac{1}{\lambda} \sum_{v_j \in \mc{\mc{N}_i}(t)}A_t(v_i,v_j)  \zeta^j_e[t] $\\
$t \gets t+1$
 }
 // Compute CMetric //\\
% Form $\cm$ using Definition~\ref{def: cmetric}\\
\For{$k=0,1,2$}{
// Compute Likelihood and Intensity // \\
$\textrm{SLE}_k(t) = \abs*{\frac{\partial \zeta(t)}{\partial t}}$\\
$\textrm{SIE}_k(t) = \abs*{\frac{\partial^2 \zeta(t)}{\partial t^2}}$
}
}
\caption{CMetric Measure outputs the Style Likelihood Estimate (SLE) and Style Intensity Estimate (SIE) for a vehicle, $u$, in a given time-period $\Delta t$. }
% \vspace{-5pt}
\end{algorithm}

% \subsection{Noise-Invariance}
