# Supplementary material for: Game-Theoretic Planning for Autonomous Driving among Risk-Aware Human Drivers
Source: arXiv:2205.00562 source file (2022-05-01)
Supplement: Supplementary file 2 [file appendixB.tex]

\section{Related Work}
\label{sec: related}
\subsection{Driving Behavior}
Driver behavior is a well-studied subject in traffic literature~\cite{def1,def2,def3,def4,def5,def6}. Due to its abstract nature, driving behavior does not lend itself to a formal definition. For example~\cite{def1,def2} describe driving behavior as driving habits that are established over a period of time. While Ishibashi et al.~\cite{def3} define driving behavior as ``an attitude, orientation and way of thinking for driving''. Despite these differences, Sagberg et al.~\cite{sagberg2015review} extract and summarize the common elements from these definitions and propose a unified definition for driving behavior as -- A global driving style that is identified through one or more specific indicators. A vehicle may be assigned a global driving style that is composed of one or more specific indicators. A global driving style refer to a generalized style of driving. For example, aggressive driving is a global style and is composed of specific indicators such as overspeeding, weaving through traffic, tailgating and so on. Conservative driving is another global style that may be composed of specific indicators such as driving at a uniform speed, braking often etc. We refer the reader to~\cite{sagberg2015review} for a detailed review.

There is a large body of research on modeling driver behavior. These approaches, however, rely on responses to questionnaires~\cite{taubman2004multidimensional,ishibashi2007indices, gulian1989dimensions,deffenbacher1994development, french1993decision} or models that need to be adjusted according to different road conditions, traffic density, geographic locations, cultures, and driver personalities~\cite{ernestref2,ernestref8,ernestref9,ernestref10,ernestref11,ernestref12,ernestref13,ernestref14,ernestref15,ernestref16, rohanref3, rohanref5, rohanref4}. Sadigh et al.~\cite{ernestref17} proposed a data-driven model based on Convex Markov Chains to predict whether a driver is paying attention while driving. Some recent approaches also utilize RL (reinforcement learning) and imitation learning techniques to teach networks to recognize various driver intentions~\cite{qi2018intent,codevilla2018end}, while others have applied RNN and LSTM-based networks to perform data-driven driver intent prediction~\cite{zyner2018recurrent,zyner2017long}. 

Feng et al.~\cite{ernestref2} proposed five driver characteristics (age, gender, personality via blood test, and education level) and four environmental factors (weather, traffic situation, quality of road infrastructure, and other cars’ behavior), and mapped them to 3 levels of aggressiveness (driving safely, verbally abusing other drivers, and taking action against other drivers). Rong et al.~\cite{rohanref3} presented a similar study but instead used different features such as blood pressure, hearing, and driving experience to conclude that aggressive drivers tailgate and weave in and out of traffic. Dahlen et al.~\cite{rohanref5} studied the relationships between driver personality and aggressive driving using the five-factor-model~\cite{big5}. Aljaafreh et al.~\cite{ernestref8} categorized driving behaviors into four classes: Below normal, Normal, Aggressive, and Very aggressive, in accordance with accelerometer data. Social Psychology studies~\cite{ernestref9,ernestref10} have examined the aggressiveness according to the background of the driver, including age, gender, violation records, power of cars, occupation, etc. Mouloua et al.~\cite{ernestref11} designed a questionnaire on subjects’ previous aggressive driving behavior and concluded that these drivers also repeated those behaviors under a simulated environment. However, the driver features used by these methods cannot be computed easily for autonomous driving in new and unknown environments, which mainly rely on visual sensors.
using current sensors like cameras or lidars. 

Several methods have analyzed driver behavior using visual and other information. Murphey et al.~\cite{ernestref12} conducted an analysis on the aggressiveness of drivers and observed that longitudinal (changing lanes) jerk is more related to aggressiveness than progressive (along the lane) jerk (i.e., rate of change in acceleration). Mohamad et al.~\cite{ernestref13} detected abnormal driving styles using speed, acceleration, and steering wheel movement, which indicated the direction of vehicles. Qi et al.~\cite{ernestref14} studied driving styles with respect to speed and acceleration. Shi et al.~\cite{ernestref15} pointed out that deceleration is not very indicative of the aggressiveness of drivers, but measurements of throttle opening, which are associated with acceleration, were more helpful in identifying aggressive drivers. Wang et al.~\cite{ernestref16} classified drivers into two categories, aggressive and normal, using speed and throttle opening captured by a simulator.

Apart from behavior prediction, some methods have been proposed for behavior modeling~\cite{yeh2008composite,helbing1995social,bera2016glmp,bera2016realtime, guy2012statistical}. In our case, we exploit the spectrum of dynamic traffic graphs to predict driver behaviors, which is complementary to these approaches and can be combined with such methods.

\subsection{Social Awareness of Autonomous Vehicles }
% With the increase in popularity of deep learning, most efforts in academic and industry research are focused towards perception problems in autonomous driving such as tracking, detection, and trajectory prediction. At the same time, relatively less research is being done to improve how AVs interact with human-driven vehicles. 
By default, AVs are designed to be conservative in nature~\cite{sa1,sa2,sa3,schwarting2019social}. The main drawback of this design is that AVs may often result in unnatural and often risky maneuvers that human drivers may not anticipate. For example, there is evidence of a Tesla Autopilot attempting to change lanes in dense traffic~\cite{dirtyTesla-gamma}. The conservative nature of the Tesla made it wait for an excessively large gap in the target lane thereby blocking the traffic behind it in the current lane. Moreover, the driver in the target lane who had slowed down to allow the Tesla to switch lanes is noticeable frustrated. Therefore, there are scenarios where autonomous vehicles need to be aggressive to appropriately interact with human drivers.

\subsubsection{Game-Theoretic Formulations of Social Awareness}

The field of socially acceptable\footnote{from here on, we use the terms socially acceptable and socially aware interchangeably} autonomous driving has started to see progress in terms of models and algorithms by combining models and algorithms from interdisciplinary fields. State-of-the-art research has currently explored game-theoretic formulations~\cite{schwarting2019social, gt1, gt2, gt3, gt4, gt5} where they model the interactions between human-driven vehicles and AVs as a non-cooperative game.

These approaches~\cite{gt2, gt4, gt5} model the agents as selfish with homogeneous decision making while considering an agent's best response given the decisions of all other agents. \cite{schwarting2019social} utilizes Social Value Orientation[cite SVO paper] to incorporate the other drivers' personality and driving styles to handle scenarios which rely on human-robot interactions, for eg., vehicle lane merging, but requires state variables like position, heading and speed for all vehicles at all time steps to solve the multi-agent game.%, which might not be possible in a real-world scenario.

\cite{gt1} proposes a closed loop feedback structure where optimal strategies are computed using dynamic programming. Even with simplified dynamics, solving this dynamical game is computationally intensive. To lower the computational intensity the strategic values are to be stored in a look-up table  requiring pre-computation for a number of scenarios which the AV might encounter, which might not be feasible.

% Write a few lines in general about the way these models work

% Write a line each about each individual work.

%  Say how your method differs from these prior approaches
