# Supplementary material for: Game-Theoretic Planning for Autonomous Driving among Risk-Aware Human Drivers
Source: arXiv:2205.00562 source file (2022-05-01)
Supplement: Supplementary file 3 [file appendixC.tex]

\section{Traffic-Graph Setup}
\label{sec: decision-making}

\label{subsec: DGG}
In this section, we describe the representation of traffic through Dynamic Geometric Graphs (DGGs).
We assume that the trajectories of all the vehicles in the video are extracted and given to our algorithm as an input.  Given this input, we first construct a DGG~\cite{waxman1988routing} at each time-step. 
% We define a dynamic geometric graph as follows:

\begin{definition}
A Geometric Graph is an undirected graph with a set of vertices $\mathcal{V}$ and a set of edges $\mc{E} \subseteq \mc{V} \times \mc{V}$ defined in the 2-D Euclidean metric space with metric function $f(x,y) = \Vts{x-y}^2$. Two vertices $v_i, v_j \in \mc{V}$ are connected if, and only if, their $f(v_i,v_j) < r$ for some constant $r$.

A Dynamic Geometric Graph (DGG) is a geometric graph with a set of vertices $\mathcal{V}(t)$ and a set of edges $\mc{E}(t)$, where $\mc{V}(t)$ and $\mc{E}(t)$ are the sets of vertices and edges as functions of time.
\end{definition}

We represent traffic at each time instance with $N$ road-agents using a DGG, where the positions of vehicles, including motorbikes and scooters, represent the vertices. In particular, we represent a vehicle position as a point in $\mathbb{R}^2$. Thus, $v_i \gets [x_i,y_i]^\top$, where $ [x_i,y_i]^\top$ is the 2-D spatial coordinates (e.g., in meters) of the $i^\textrm{th}$ vehicle in the global coordinate frame.
For a DGG, $\mc{G}$, the adjacency matrix, $A \in \mathbb{R}^{N \times N}$ is given by,

\begin{equation}
% \resizebox{0.7\columnwidth}{!}{
A(i,j)=
     \begin{cases}
      d(v_i,v_j) & \text{if $d(v_i,v_j) < \mu,i \neq j$ },\\
    %   -1 &\quad\text{if $e_{ij} \in \mc{E}$}, \\
      0 &\text{otherwise.}
     \end{cases}
    %  }
     \label{eq: similarity_function}
\end{equation}
\noindent where $d(v_i,v_j)$ denotes the Euclidean distance between the $i^\textrm{th}$ and $j^\textrm{th}$ vehicles, and $\mu$ is a distance threshold parameter.
% We discuss its implementation in Section~\ref{sec: experiments}.
For an adjacency matrix $A$ at each time instance, the corresponding degree matrix $D \in \mathbb{R}^{N \times N}$ is defined as a diagonal matrix with main diagonal $D(i, i) = \sum_{j=1}^N A(i, j)$ and 0 otherwise. 
Further, the symmetric Laplacian matrix can be obtained by subtracting $A$ from $D$, 

% \vspace*{-5pt}
\begin{equation}
% \resizebox{0.6\columnwidth}{!}{
L(i,j) =
     \begin{cases}
      D(i,i)  &\text{if $i=j$},\\
      -e^{-d(v_i,v_j)} &\text{if $d(v_i,v_j) < \mu$}, \\
      0 &\text{otherwise.}
     \end{cases}
    %  }
\end{equation}
The laplacian matrix for each time-step is correlated with the laplacian matrices for all previous time-steps. If the laplacian matrix at a time instance $t$ be denoted as $L_t$. Then, the laplacian matrix for the next time-step, $L_{t+1}$ is given by the following update,

\begin{equation}
% \resizebox{0.4\columnwidth}{!}{
L_{t+1} =
\left[
\begin{array}{c|c}
L_{t} \Bstrut & 0 \Bstrut\\
\hline
0 \Tstrut & 1
\end{array}
\right] + \delta\delta^\top,
% }
\label{eq: A_update}
\end{equation}

\noindent where $\delta \in \bb{R}^{d \times 2} $ is a sparse matrix with $\Vts{\delta}_0 \ll n$. The update rule in Equation~\ref{eq: A_update} enforces a vehicle to add edges connections to new vehicles while retaining edges with previously seen vehicles. $L_t$ is updated in-place with time and is reset to a zero matrix once the number of vehicles crosses some fixed $N$.

The spectrum $U$ of the Laplacian matrix $\mc{L}$ can be used to compute the topology of a vertex. Let $w_i \in \mathbb{R}^{n}$ denote the $i^{\textrm{th}}$ column of the matrix $\mc{L} U$. Then the $j^{\textrm{th}}$ entry of $w_i$ is given by,
%, where $U \in \mathbb{R}^{n\times k}$ is the eigenvector matrix, that is, $w_i = \li u_i$
% \vspace*{-6pt}
\begin{equation*}
w_i(j) = D(j,j)u_i(j) - \sum u_i(k) = \sum \brr{u_i(j)-u_i(k)}.
\label{eq: w}
\end{equation*}
% \vspace*{-1pt}
\noindent Thus, the $j^{\textrm{th}}$ entry of $w_i$ equals the sum of edge values of all edges with $v_j$ as the common node. Since the arrangement of vertices depend on the edge lengths between them, this determines the topology of the graph. 
% The presence of a non-zero value in the $j^\textrm{th}$ row of $\delta$ indicates that the $j^\textrm{th}$ road-agent has formed an edge connection with a new vehicle, that has been added to the current DGG. The size of $L_t$ is fixed for all time $t$ and is initialized as a zero matrix of size $N$x$N$, where $N$ is max number of agents. $L_t$ is updated in-place with time and is reset to a zero matrix once the number of vehicles crosses $N$. The diagonal elements of the Laplacian matrix in Equation~\ref{eq: A_update} is used by the degree centrality to characterize overspeeding~\ref{Subsec: Centrality}.
