# Supplementary material for: Game-Theoretic Planning for Autonomous Driving among Risk-Aware Human Drivers
Source: arXiv:2205.00562 source file (2022-05-01)
Supplement: Supplementary file 4 [file appendixE.tex]

\section{Additional Details on Datasets and TDE Metric}
\label{app: dataset}

\subsection{Datasets}

One of the main issues that arise in the evaluation of driving behavior research is the lack of publicly available large-scale datasets for driving behaviors that specifically contain labels for aggressive and conservative vehicles. In light of these limitations, we create driver behavior annotations using Algorithm~\ref{alg: ex} on videos in large-scale trajectory prediction and tracking datasets~\cite{Argoverse,lyft2019,ma2018trafficpredict}. Our new dataset consists of videos of dense urban traffic with annotated trajectories from different geographic regions such as U.S. and Singapore. We directly use the raw trajectory data from these datasets without any pre-processing or filtering step. We describe the exact annotation procedure in the following subsection.
% The Argoverse motion forecasting data consists of 324,557 video segments of 5 seconds each. The total video length is 320 hours. The dataset contains traffic videos recorded in Miami (204 kilometers) and Pittsburgh (6 kilometers). The format of the data includes the timestamp, road-agent I.D., road-agent type, the spatial coordinates, and the location.

\subsection{Annotation Procedure}

From existing large-scale autonomous driving datasets~\cite{Argoverse,lyft2019,ma2018trafficpredict}, we extract a total of $P$ videos that are annotated by $M$ participants via a crowd-sourced user study. For each video, the final ground-truth annotation (or label) is the expected value of the frame at which the ego-vehicle is most likely to be executing an aggressive style. This is denoted as $\EX[T]$. The goal for any driver behavior prediction model should be to predict the aggressive style at a time-stamp as close to $\EX[T]$ as possible. The implied difference in the two time-stamps is measured by the TDE metric.

\begin{algorithm}
    \SetKwInOut{Input}{Input}
    \SetKwInOut{Output}{Output}
\SetKwComment{Comment}{$\triangleright$\ }{}
\SetAlgoLined
\Input{$M$ participants, set of starting frames $S = \{s_1, s_2, \ldots, s_M\}$, set of ending frames $E = \{e_1, e_2, \ldots, e_M\}$ }
\Output{$\EX[T]$ for a video}
$s^* = \min S$\\
$e^* = \max E$\\
Initialize a counter $c_t = 0$ for each frame $t \in [s^*, e^*]$\\
\For {$t \in [s^*, e^*]$}{
\If{$t \in [s_m, e_m]$}{
$c_t \gets c_t + 1$
}
$\mathcal{P}(T=t) = c_t $
}
$\EX[T] = \sum_t tc_t$, $t = s^*, s^*+1, \ldots, e^*$
\caption{Computing $\EX[T]$ for each video in a dataset.}
\label{alg: ex}
% \vspace{-5pt}
\end{algorithm}

The TDE metric is computed by Equation~\ref{eq: TDE}. Here, $t_\textrm{SLE} =  \argmax_{t \in \Delta t}{\textrm{SLE}(t)}$, as explained in Section~\ref{sec: metric}. We use Algorithm~\ref{alg: ex} for computing $\EX[T]$. For each video, $M$ participants marked the starting and end frames for the time-period during which a vehicle is observed to be executing an aggressive maneuver. For each video, we end up with $S = \{s_1, s_2, \ldots, s_M\}$ and $E = \{e_1, e_2, \ldots, e_M\}$ start and end frames, respectively. We extract the overall start and end frame by finding the minimum and maximum value in $S$ and $E$, respectively. We denote these values as $s^*$ and $e^*$. Initialize a separate counter, $c_t$, for each frame $t \in [s^*, e^*]$. Increment a counter by $1$, if $t \in [s_m, e_m]$. This then results in $\mathcal{P}(T)$. The $\EX[T]$ of $\mathcal{P}(T)$ can be then computed using the standard definition of expectation of a discrete probability mass function. We can apply algorithm~\ref{alg: ex} separately for each video in the dataset.
