# Supplementary material for: Game-Theoretic Planning for Autonomous Driving among Risk-Aware Human Drivers
Source: arXiv:2205.00562 source file (2022-05-01)
Supplement: Supplementary file 5 [file appendixF.tex]

\section{Additional Details for Simulation Environment}
\label{app: simulation_details}

We use the Highway-Env simulator~\cite{leurent2019social} that is developed using PyGame~\cite{pygame}. The simulator consists of a 2D environment where vehicles are made to drive along a multi-lane highway using the Bicycle Kinematic Model~\cite{polack2017kinematic} as the underlying motion model. The linear acceleration model is based on the Intelligent Driver Model(IDM)~\cite{treiber2000congested} and is computed via the following kinematic equation,
\begin{equation}
    \dot v_{\alpha} = a\begin{bmatrix}1 - (\frac{v_{\alpha}}{v_0^{\alpha}})^4 - (\frac{s^*(v_{\alpha}, \Delta v_{\alpha})}{s_{\alpha}})^2\end{bmatrix}
    \label{eq: IDM_acc}
\end{equation}

\noindent Here, the linear acceleration, $\dot v_{\alpha}$, is a function of the velocity $v_{\alpha}$, the net distance gap $s_{\alpha}$ and the velocity difference $\Delta v_{\alpha}$ between the ego-vehicle and the vehicle in front. Equation~\ref{eq: IDM_acc} is a combination of the acceleration on a free road $\dot v_{free} = a[1 - (v/v_0)^{4}]$ (\textit{i.e.} no obstacles) and the braking deceleration, $-a(s^*(v_\alpha,\Delta v_\alpha)/s_\alpha)^2$ (\textit{i.e.} when the ego-vehicle comes in close proximity to the vehicle in front). The deceleration term depends on the ratio of the desired minimum gap ($s^*(v_\alpha,\Delta v_\alpha)$) and the actual gap ($s_{\alpha}$), where $s^* (v_\alpha,\Delta v_\alpha)= s_0 + vT + \frac{v\Delta v}{2\sqrt{ab}}$. $s_0$ is the minimum distance in congested traffic, $vT$ is the distance while following the leading vehicle at a constant safety time gap $T$, and $a,b$ correspond to the comfortable maximum acceleration and comfortable maximum deceleration, respectively. 

The lane changing behavior is based on the MOBIL~\cite{kesting2007general} model. According to this model, there are two key parameters when considering a lane-change:
\begin{enumerate}
    \item \textit{Safety Criterion}: This condition checks if, after a lane-change to a target lane, the ego-vehicle has enough room to accelerate. Formally, we check if the deceleration of the successor $a_\textrm{target}$ in the target lane exceeds a pre-defined safe limit $b_{safe}$:
    \begin{equation*}
        a_\textrm{target} \geq -b_{safe}
    \end{equation*}
    
    \item \textit{Incentive Criterion}: This criterion determines the total advantage to the ego-vehicle after the lane-change, measured in terms of total acceleration gain or loss. It is computed with the formula,
    
    \begin{equation*}
    \tilde{a}_\textrm{ego} - a_\textrm{ego} + p(\tilde{a}_n - a_n + \tilde{a}_o - a_o) > \Delta a_{th}
    \end{equation*}
    where $\tilde{a}_\textrm{ego} - a_\textrm{ego}$ represents the acceleration gain that the ego-vehicle would receive after to the lane change. The second term denotes the total acceleration gain/loss of the immediate neighbours (the new follower in the target, $a_n$, and the original follower in the current lane, $a_o$) weighted with the politeness factor, $p$. By adjusting $p$ the intent of the drivers can be changed from purely egoistic ($p=0$) to more altruistic ($p=1$). We refer the reader to~\cite{kesting2007general} for further details.
\end{enumerate}

\noindent The lane change is executed if both the safety criterion is satisfied, \textit{and} the total acceleration gain is more than the defined minimum acceleration gain, $\Delta a_{th}$.

The original simulator proposed by Leurent et al.~\cite{leurent2019social} generates homogeneous agents that are parameterized by default to behave conservatively. We modified the simulation parameters and designed two different classes of heterogeneity (See Figure~\ref{fig: simulator_figs}) to produce both conservative (blue agents) and aggressive vehicles (green agent). The parameters used to generate the two classes of vehicles are given in Table~\ref{tab: parameters}.
\begin{table}[h]
\caption{IDM and MOBIL parameters used for Conservative and Aggressive vehicle classes}
\centering
\resizebox{\columnwidth}{!}{%
\begin{tabular}{clcc} 
\toprule
Model & Parameter \Tstrut & Conservative \Bstrut &   Aggressive \\
\hline
\multirow{4}{*}{IDM}& Time gap ( $T$) \Tstrut & 1.5s      & 1.2s \\
 &Min distance ($s_0$) & 5.0 $m$ & 2.5 $m$ \\
&Max comfort acc. ($a$)     & 3.0 $m/s^2$ & 6.0 $m/s^2$\\
&Max comfort dec. ($b$) & 6.0 $m/s^2$               &  9.0 $m/s^2$ \\
\midrule
\multirow{3}{*}{MOBIL}& Politeness ($p$) & 0.5     & 0\\
& Min acc gain ($\Delta a_{th}$) & 0.2 $m/s^2$ & 0 $m/s^2$ \\
& Safe acc limit ($b_{safe}$) & 3.0 $m/s^2$ & 9.0 $m/s^2$\\
\bottomrule
\end{tabular}
}
\label{tab: parameters}
\vspace{-10pt}
\end{table}

Additionally, the desired velocity $v_0$ was set to $25$ meters per second and $40$ meters per second for the conservative and aggressive vehicle classes, respectively. Finally, the desired velocities for the conservative vehicles were uniformly distributed with a variation of {$\pm$10\%} to increase the heterogeneity in the simulation environment.
