# Supplementary material for: Game-Theoretic Planning for Autonomous Driving among Risk-Aware Human Drivers
Source: arXiv:2205.00562 source file (2022-05-01)
Supplement: Supplementary file 6 [file appendixG.tex]

\section{Proofs to Theorems IV.1 and IV.2}

\begin{theorem}
For each active agent $a_i \in \mathcal{A}$ at a traffic intersection, roundabout, or during merging, bidding $b_i = \zeta_i$ is the dominant strategy. 
\label{thm: incentive_compatibility}
\end{theorem}

% \noindent We defer the proof to the supplementary material.
\begin{proof}
Recall that the $k^\textrm{th}$ highest bidder ($k^\textrm{th}$ most aggressive agent) is allocated the $k^\textrm{th}$ position in the turn-based ordering $\sigma$. Each turn $\sigma_k$ is associated with a time reward $\alpha_k = \frac{1}{t_k}$. Then according to Equation~\ref{eq: utility_template}, the overall utility achieved by the $k^\textrm{th}$ most aggressive traffic-agent is,  

\begin{equation}
  u_k (b_k) =  b_k \left( \frac{1}{t_k} \right) - \sum_{j=k}^K b_{j+1} \left(\frac{1}{t_j} - \frac{1}{t_{j+1}} \right).
    \label{eq: utility}
\end{equation}

\noindent We sort the $K$ highest bids received in the following order: $b_1 > b_2 > \ldots > b_K$. In order to show that $b_k = \zeta_k$ is the dominant strategy, it is sufficient to show that over-bidding ($\bar b_k = b_{k-1}$) and under-bidding ($\bar b_k = b_{k+1}$) both result in a lower utility than $u_k$. We proceed by individually analyzing each case.

\noindent \textbf{Case 1: Over-bidding ($\bar b_k = b_{k-1} > b_k$):} We have 

\begin{equation*}
\begin{split}
    &\bar u_k (\bar b_k) = \\
     &b_{k-1} \left( \frac{1}{t_{k-1}} \right) - b_k \left( \frac{1}{t_{k-1}} - \frac{1}{t_{k}} \right ) - \sum_{j=k}^K b_{j+1} \left(\frac{1}{t_j} - \frac{1}{t_{j+1}} \right). \\
\end{split}    
\end{equation*}

\noindent We observe that  $\bar u_k (\bar b_k) - u_k (b_k) =  b_{k-1} \left( \frac{1}{t_{k-1}} \right)  - b_k \left( \frac{1}{t_{k-1}}\right ) < 0$ since $b_k > b_{k-1}$. 

\noindent \textbf{Case 2: Under-bidding ($\bar b_i = b_{i+1} < b_i$):} We have 

\begin{equation*}
    \bar u_k (\bar b_k) =  b_{k+1} \left( \frac{1}{t_{k+1}} \right) - \sum_{j=k+1}^K b_{j+1} \left(\frac{1}{t_j} - \frac{1}{t_{j+1}} \right)
\end{equation*}

\noindent Observe that  $u_k (b_k) - \bar u_k (\bar b_k) =  b_{i} \left( \frac{1}{t_k} \right)  - b_{k+1} \left( \frac{1}{t_{k+1}}\right ) + b_{k+1} \left( \frac{1}{t_{k}} - \frac{1}{t_{k+1}}\right ) $. This simplifies to $b_{k} \left( \frac{1}{t_k} \right) - b_{k+1} \left( \frac{1}{t_{k}} \right) > 0$ since $b_k > b_{k+1}$.
\vspace{5pt}
\end{proof}

\begin{theorem}
For each active agent $a_i \in \mathcal{A}$, bidding $b_i = \zeta_i$ maximizes social welfare. 
\label{thm: Welfare_Maximizing}
\end{theorem}

% \noindent We defer the proof to the supplementary material.

\begin{proof}
Our proof is based on induction. We begin with the base case with the most aggressive agent (highest bidder). Recall that after sorting, we have agents in decreasing order of aggressiveness \textit{i.e.} $\zeta_1 > \zeta_2>\ldots> \zeta_n$ and $\frac{1}{t_1} > \frac{1}{t_2}>\ldots> \frac{1}{t_k}$. Therefore, we have that $\frac{\zeta_1}{t_1}$ is maximum. Next, consider the hypothesis that the sum $\sum_{j=1}^k\frac{\zeta_j}{t_j}$ is maximum up to the $k^\textrm{th}$ highest bidder. Then the inductive step is to prove that $\sum_{j=1}^{k+1} \frac{\zeta_j}{t_j}$ is maximum. 

Observe that $\sum_{j=1}^{k+1} \left( \frac{\zeta_j}{t_j}\right) = \sum_{j=1}^k \left(\frac{\zeta_j}{t_j}\right) + \frac{\zeta_{k+1}}{t_{i+1}}$. Note that the first term on the RHS is maximum from hypothesis. Then $\zeta_{k+1} > \zeta_{k+2} > \zeta_{k+3}>\ldots> \zeta_n $ and $\frac{1}{t_{k+1}} > \frac{1}{t_{k+2}}>\ldots> \frac{1}{t_K}$ implies that $\frac{\zeta_{k+1}}{t_{k+1}}$ is maximum.
\vspace{5pt}
\end{proof}

\section{Comparison with prior work}

There are two key benefits of our approach over prior work. First, \model~produces better results in terms of fewer collisions and deadlocks with \textit{no} restrictions and assumptions on the modeling of traffic-agents. Our maximum improvement is over the approach by Roh et al.~\cite{roh2020multimodal} with up to $30\%$ reduction in collisions with $4$ agents on a $4-$way traffic intersection. Game-theoretic approaches~\cite{li2020game,tian2020game} place implausible restrictions on the actions and objectives of active agents. For example, Li et al.~\cite{li2020game} formulate traffic intersection planning as a stackelberg leader-follower game in which one agent is assumed to act first (leader) and the other agent (follower) will react accordingly. Tian et al.~\cite{tian2020game} use a recursive $k-$level game-theoretic approach in which complex strategies for agents at each level are derived from previous levels. However, all agents except the ego-agent at the first level are assumed to be static. DRL-based methods~\cite{isele2018navigating, liu2020decision, Kai2020AMR} learn a navigation policy using the notion of expected reward received by an agent from taking a particular action in a particular state. This policy is learned from trajectories obtained via traffic simulators using Q-learning~\cite{dql} and is very hard as well as expensive to train. In practice, DRL-based planning methods often do not generalize well to different environments and it is hard to provide any guarantees. Finally, deep learning-based methods~\cite{roh2020multimodal} train a recurrent neural network for trajectory prediction and are also susceptible to complex environments or different behavior of drivers. In contrast to all of the above, \model~places no restrictions on the objective functions of other traffic-agents and generalizes to different traffic scenarios.

The second key benefit of our approach over prior methods is that our results are game-theoretically optimal for $n$ agents in $n-$way traffic intersections. That is, as $n$ increases, our approach can scale accordingly and we can still guarantee $0$ collisions and deadlocks from a planning standpoint. We observe that the number of collisions increases for the approaches of Li et al.~\cite{li2020game} and Roh et al.~\cite{roh2020multimodal} as the number of agents and service lanes in the intersections increase. 

\section{Demonstrating \model~with Human Drivers}

\input{NeuRIPS2020/img/Real World}
