# Supplementary material for: Game-Theoretic Planning for Autonomous Driving among Risk-Aware Human Drivers
Source: arXiv:2205.00562 source file (2022-05-01)
Supplement: Supplementary file 7 [file appendixH.tex]

\section{NP-complete (\textcolor{red}{\textbf{TO DO}})}

In this paper, we described a method to compute game-theoretically optimal turn-based orderings which help in navigating traffic scenes in a collision- and deadlock-free way. $\sigma_{\textsc{opt}}$ is based on driver behavior. Driver behavior is what we are going to refer to as an attribute.

\begin{definition}
An attribute is a mapping $\bm{\Lambda}: \mathcal{A} \rightarrow \mathbb{R}$.
\end{definition}

\noindent $\bm{\Lambda}$ is an element of an infinitely countable set. We define such a set as $\bm{\Upsilon} = \{ \bm{\Lambda}_1, \bm{\Lambda}_2, \ldots, \}$, where $\bm{\Lambda}$ is indexed by the natural numbers. Then the mapping corresponding to driver behavior may be indexed by some constant $d \in \mathbb{N}$ to produce a mapping $\bm{\Lambda}_d$.

Now the natural question may be asked - what if we were to choose a different attribute than driver behavior, (any $j \neq d \in \mathbb{N}$)? Can a different sorting strategy be used to sort drivers and therefore come up with a different turn-based ordering that is also game-theoretically optimal?

We will show that finding the attribute that results in a game-theoretically optimal turn-based ordering is NP-complete.

\subsection{Model $\mathcal{M}$}
\begin{itemize}
    \item Given $N$ human drivers, we want to identify first-goers, second-goers, $\ldots$, $k^\textrm{th}$-goers etc. This amounts to making $k$ clusters, $\mathcal{C}_1,\mathcal{C}_2,\ldots,\mathcal{C}_k$, where $\mathcal{C}_i$ consists of the drivers who will move on the $i^\textrm{th}$ turn while maintaining game-theoretic optimality.
    
    \item Given a set of attribute mappings $\bm{\Upsilon} = \{ \bm{\Lambda}_1, \bm{\Lambda}_2, \ldots\}$ where $\bm{\Lambda}_j: \mathcal{A} \rightarrow \mathbb{R}$. No other information is known about an agent. $\bm{\Lambda}_j(a_i)$ can be computed in polynomial time.

    \item We want to find the attribute mapping, say $\bm{\Lambda}_j \in \bm{\Upsilon}$, such that $\bm{\Lambda}_j(a_1) > \bm{\Lambda}_j(a_1)>\ldots>\bm{\Lambda}_j(a_k) \ \forall a_1,a_2,\ldots,a_k \in \mathcal{C}_1,\mathcal{C}_2,\ldots,\mathcal{C}_k$. 
    
    \item Assume fixed number of clusters ($k \geq 2$) but number of agents ($N$) is part of input.
    
    \item $P(\bm{\Lambda}_j (a_i) | a_i)$ is unknown.
    
\end{itemize}

\begin{figure}[t]
    \centering
    \includegraphics[width = \linewidth]{NeuRIPS2020/img/Appendix/NP-complete digram.png}
    \caption{Attributes in \model.}
    \label{fig: np-complete}
\end{figure}

\subsection{Result}

\begin{theorem}
Finding a game-theoretically optimal attribute is NP-complete.
\end{theorem}

\begin{proof}
We reduce \texttt{SAT} to our model.  Each cluster is a circuit composed of the corresponding clause.

\begin{enumerate}

    \item $\mathcal{M} \in \textrm{NP}$. Proof - Given $N$ agents, $k$ clusters, and an attribute mapping $\bm{\Lambda}_j, j\in \mathbb{N}$, checking the mapping takes $\bigO{\floor*{\frac{N}{k}}^{k}}$. Note that $\mathcal{M}$ is $\texttt{EXPTIME}$ if $k$ is not fixed.

    \item $\phi \implies \mathcal{M}$: Let $\phi$ be satisfied by $\hat j = x_1x_2\ldots x_n$ and let $j$ be the decimal form of $\hat j$. The attribute map is $\bm{\Lambda}_j(a_i) = (j + k - i)*\texttt{bool}(\mathcal{C}_i) \in \mathbb{R} \ \forall a_i \in \mathcal{C}_i, i \in [1,k]$. Therefore, $\bm{\Lambda}_j(a_i)$ can be either $j+k-i$ or $0$. Each agent in $\mathcal{C}_i$ is represented by $a_i \gets (l, (j+k-i)*\texttt{bool}(\mathcal{C}_i))$ where $l$ represents the literal in the $i^\textrm{th}$ clause. 
    
    Now, $j$ satisfying $\phi$ implies that there exists a game-theoretically optimal attribute mapping $\bm{\Lambda}$ that fits model $\mathcal{M}$. Indeed, such a mapping is $\bm{\Lambda}_j(a_i) = (j + k - i)*\texttt{bool}(\mathcal{C}_i) \in \mathbb{R} \ \forall a_i \in \mathcal{C}_i, i \in [1,k]$. To see why, pick any agent from $\mathcal{C}_1$. Since every clause is true, $\bm{\Lambda}_j(a_1) = j+k-1$. Similarly, any agent from $\mathcal{C}_2$ will have an attribute value of $j+k-2 < j+k-1$. So on up til $\mathcal{C}_k$ in which each agent has attribute value $j$.
    
    \item $\mathcal{M} \implies \phi$: Assume there exists a game-theoretically optimal attribute $\bm{\Lambda}_j$. $\hat j = j$ if $j\in [1,2^n]$ else $\hat j = j\bmod 2^n$. Then $\bm{\Lambda}_j(a_1) > \bm{\Lambda}_j(a_2)>\ldots>\bm{\Lambda}_j(a_k) \ \forall a_1,a_2,\ldots,a_k \in \mathcal{C}_1,\mathcal{C}_2,\ldots,\mathcal{C}_k$ and $j\in \mathbb{N}$. This automatically implies each cluster has a truth value of $1$. To see why, assume that $\phi$ is not satisfied. Then there exist one or more clusters whose truth value is $0$. Assume that such a cluster is $\mathcal{C}_i$. Then each agent in $\mathcal{C}_i$ has an attribute value of $0$ contradicting the game-theoretic optimality ($0 > j+k-(i+1)$ is a contradiction since $j\in \mathbb{N}$ and $k \geq 2$). Therefore, each clause/cluster has a truth value of $1$ implying $\phi$ is satisfied.
    
    % To obtain $\hat j$, note that if $\hat j = j$ if $j\in [1,2^n]$. Otherwise, $\hat j = j\mod 2^n$
\end{enumerate}

% \noindent Think of the solution code as ``lighting up'' the clusters (setting them to 1). The problem is we do not know which attribute results in the desired order (lights up all the clusters). 
\end{proof}

\noindent This means that given a traffic scenario such as an intersection or roundabout with $k$ arms that requires the interaction of $N$ agents (nothing known about them), unless $P = NP$, collision- and deadlock-free navigation cannot be guaranteed without relaxing some of the constraints or making assumptions heuristically.

\subsection{Heuristic algorithms to solve $\mathcal{M}$}

Recall that the end goal is to compute $\sigma_{\textsc{opt}}$ which, as per the discussion in this section, depends on the optimal attribute mapping $\bm{\Lambda}_j$. We have proven that finding the value of $j$ is NP-complete. However, one can design heuristic algorithms to solve $\mathcal{M}$. The basic premise of such an algorithm is to relax some of the constraints above associated with $\mathcal{M}$.

For example, \model~is one such heuristic algorithm where we relax the last constraint, \textit{i.e.}, we use an attribute mapping with a known probability distribution, $P(\bm{\Lambda}_j (a_i) | a_i)$. Consider an aggressive agent $a_{\textsc{aggressive}}$. Then it is known with high probability that $\bm{\Lambda}_j (a_{\textsc{aggressive}}) = t$ for some fixed $t$. Monetary-based auction methods are another instance of a heuristic multi-agent game-theoretic planning algorithms for computing game-theoretical turn-based orderings. In these type of methods, it is assumed that agents are given a known monetary budget. Consequently, the mapping is provided by an oracle and is not known to be computed in polynomial time. Such auctions work by relaxing the second constraint.
