# Supplementary material for: Game-Theoretic Planning for Autonomous Driving among Risk-Aware Human Drivers
Source: arXiv:2205.00562 source file (2022-05-01)
Supplement: Supplementary file 8 [file appendixD.tex]

\section{Additional Results}
\label{app: additional_results}
